# Supplementary material for: Reuse and Diffuse: Iterative Denoising for Text-to-Video Generation
Source: arXiv:2309.03549 source file (2023-09-07)
Supplement: Supplementary file 1 [file appendix.tex]

\todo{appendix here}
